# Supplementary material for: Quantized Compressed Sensing by Rectified Linear Units
Source: arXiv:1911.07816 source file (2021-03-26)
Supplement: Supplementary file 1 [file sec_AppendixOLD.tex]

\section{Probabilistic estimates}

\begin{lemma}[Paley-Zygmund]
Let $Z$ denote a positive random variable, such that $(\E Z^p)^{1/p} < \infty$. Then, for $\frac{1}{p} + \frac{1}{q} = 1$,
\begin{equation}
    \Pb(Z \geq \theta \E Z) \geq (1-\theta)^q \frac{(\E Z)^q}{(\E Z^p)^{q/p}} \; .
\end{equation}
\end{lemma}
\begin{proof}
We observe that by H\"older's inequality
\begin{align*}
    \E Z &= \E Z \1_{Z \geq \alpha} + \E Z \1_{z \leq \alpha} \\
    &\leq (\E Z^p)^{1/p} \Pb(Z \geq \alpha)^{1/q} + \alpha \; . \\
\end{align*}
By rearranging the above inequality, we find
\begin{equation*}
    \Pb(Z \geq \alpha) \geq \frac{(\E Z - \alpha)^q}{(\E Z^p)^{q/p}} \; .
\end{equation*}
Choosing $\alpha = \theta \E Z$, it follows that
\begin{equation}
    \Pb(Z \geq \theta \E Z) \geq (1-\theta)^q \frac{(\E Z)^q}{(\E Z^p)^{q/p}} \; .
\end{equation}
This is the desired estimate.
\end{proof}

\section{Expectation bound}

\begin{lemma} \label{expectation} Let $\x,\z\in R B^n_2$. If 
\begin{equation}
    \la^2 \gtrsim R^2 L^2 \log(4L),
\end{equation}
then
\begin{equation*}
    \E \L_{q(\x)}(\z)\geq \frac{\|\x-\z\|_2^2}{8\la}.
\end{equation*}
\end{lemma}
\begin{proof} We have the following lower bound:
\begin{align*}
\E \L_{q(\x)}(\z)&=\E \relu{-\sign(\inner{\a}{\x}+\tau)(\inner{\a}{\z}+\tau)}\\
&=\E \left( 1_{\sign(\inner{\a}{\x}+\tau)\neq \sign(\inner{\a}{\z}+\tau)}|\inner{\a}{\z}+\tau|\right)\\
&\geq \E \left(1_{|\inner{\a}{\x}|\leq \la}
1_{|\inner{\a}{\z}|\leq \la}1_{\sign(\inner{\a}{\x}+\tau)\neq \sign( \inner{\a}{\z}+\tau)}|\inner{\a}{\z}+\tau|\right)\\
&=\E_a \left(1_{|\inner{\a}{\x}|\leq \la}
1_{|\inner{\a}{\z}|\leq \la} \E_\tau ( 1_{\sign(\inner{\a}{\x}+\tau)\neq \sign(\inner{\a}{\z}+\tau)}|\inner{\a}{\z}+\tau|)\right).\\
\end{align*}
Next, conditioned on the event $|\inner{\a}{\x}|\leq \la$ and $|\inner{\a}{\z}|\leq \la$, we compute
\begin{align*}
    \E_\tau ( 1_{\sign(\inner{\a}{\x}+\tau)\neq \sign(\inner{\a}{\z}+\tau)}|\inner{\a}{\z}+\tau|)
    &= \E_\tau ( 1_{\inner{\a}{\x}+\tau \leq 0 \leq   \inner{\a}{\z}+\tau}(\inner{\a}{\z}+\tau))\\
    &\quad +\E_\tau ( 1_{\inner{\a}{\z}+\tau \leq 0 \leq   \inner{\a}{\x}+\tau}(-\inner{\a}{\z}-\tau))\\
    &= \E_\tau ( 1_{- \inner{\a}{\z}\leq \tau \leq -\inner{\a}{\x}}(\inner{\a}{\z}+\tau))\\
    &\quad +\E_\tau ( 1_{- \inner{\a}{\x}\leq \tau \leq -\inner{\a}{\z}}(-\inner{\a}{\z}-\tau)).
\end{align*}
We distinguish the cases $-\inner{\a}{\z}\leq -\inner{\a}{\x}$, and $-\inner{\a}{\x}\leq -\inner{\a}{\z}$.
If $-\inner{\a}{\z}\leq -\inner{\a}{\x}$, then 
\begin{align*}
 \E_\tau ( 1_{\sign(\inner{\a}{\x}+\tau)\neq \sign(\inner{\a}{\z}+\tau)}|\inner{\a}{\z}+\tau|)
 &=\E_\tau ( 1_{- \inner{\a}{\z}\leq \tau \leq -\inner{\a}{\x}}(\inner{\a}{\z}+\tau))\\
 &=\frac{1}{2\la}\int_{-\inner{\a}{\z}}^{-\inner{\a}{\x}} (\inner{\a}{\z}+t)dt\\
 &=\frac{1}{2\la}\left[\inner{\a}{\z}t + \frac{1}{2}t^2\right]_{-\inner{\a}{\z}}^{-\inner{\a}{\x}}\\
 &=\frac{1}{4\la}\inner{\a}{\x-\z}^2.
\end{align*}
If $-\inner{\a}{\x}\leq -\inner{\a}{\z}$, then
\begin{align*}
 \E_\tau ( 1_{\sign(\inner{\a}{\x}+\tau)\neq \sign(\inner{\a}{\z}+\tau)}|\inner{\a}{\z}+\tau|)
 &=\E_\tau ( 1_{- \inner{\a}{\x}\leq \tau \leq -\inner{\a}{\z}}(-\inner{\a}{\z}-\tau))\\
 &=\frac{1}{2\la}\int_{-\inner{\a}{\x}}^{-\inner{\a}{\z}} (-\inner{\a}{\z}-t)dt\\
 &=\frac{1}{2\la}\left[-\inner{\a}{\z}t - \frac{1}{2}t^2\right]_{-\inner{\a}{\x}}^{-\inner{\a}{\z}}\\
 &=\frac{1}{4\la}\inner{\a}{\x-\z}^2.
\end{align*}
Summarizing these estimates yields that on the event $|\inner{\a}{\x}| \leq \lambda, |\inner{\a}{\z}|
\leq \lambda$ we have
\begin{equation} \label{conditioned_expectation}
     \E_\tau ( 1_{\sign(\inner{\a}{\x}+\tau)\neq \sign(\inner{\a}{\z}+\tau)}|\inner{\a}{\z}+\tau|)
        = \frac{1}{4\la}\inner{\a}{\x-\z}^2 \; .
\end{equation}
Therefore
\begin{align*}
 \E \L_{q(\x)}(\z)&\geq \frac{1}{4\la} \E \left(1_{|\inner{\a}{\x}|\leq \la}
1_{|\inner{\a}{\z}|\leq \la}\inner{\a}{\x-\z}^2\right).  
\end{align*}
We estimate using the Cauchy-Schwarz inequality:
\begin{align*}
  &\E \left(1_{|\inner{\a}{\x}|\leq \la}
1_{|\inner{\a}{\z}|\leq \la}\inner{\a}{\x-\z}^2\right)\\
&=\E\inner{\a}{\x-\z}^2 - \E \left(1_{\{|\inner{\a}{\x}|> \la\; \lor\; 
|\inner{\a}{\z}|> \la\}}\inner{\a}{\x-\z}^2\right)\\
&\geq \E\inner{\a}{\x-\z}^2 - \left(\E 1_{\{|\inner{\a}{\x}|> \la\; \lor\; 
|\inner{\a}{\z}|> \la\}} \right)^{1/2}\left(\E\inner{\a}{\x-\z}^4\right)^{1/2}\\
&= \|\x-\z\|_2^2 - \Pb(|\inner{\a}{\x}|> \la\; \lor\; 
|\inner{\a}{\z}|> \la)^{1/2} \norm{\inner{\a}{\x-\z}}{L_4}^2.
\end{align*}
Observe that for any $\x\in R B^n_2$,
\begin{align*}
    \Pb(|\inner{\a}{\x}|> \la)\leq 2\exp(-c\la^2/L^2\|\x\|_2^2)\leq 2\exp(-c\la^2/L^2R^2),
\end{align*}
where we have used that 
$\norm{\inner{\a}{\x}}{\psi_2}\lesssim L\norm{\inner{\a}{\x}}{L_2}=L\|\x\|_2$.
Further, it holds 
\begin{equation*}
\norm{\inner{\a}{\x-\z}}{L_4}\leq 2L\norm{\inner{\a}{\x-\z}}{L_2}=2L\|\x-\z\|_2.
\end{equation*}
All together, we obtain
\begin{align*}
    \E \L_{q(\x)}(\z)&\geq \frac{1}{4\la}\left( \|\x-\z\|_2^2 - \Pb(|\inner{\a}{\x}|> \la\; \lor\; 
|\inner{\a}{\z}|> \la)^{1/2} \norm{\inner{\a}{\x-\z}}{L_4}^2 \right)\\
&\geq \frac{1}{4\la}\left( \|\x-\z\|_2^2 - 8L^2\exp(-c\la^2/L^2R^2) \|\x-\z\|_2^2\right)\\
&\geq \frac{1}{8\la}\|\x-\z\|_2^2,
\end{align*}
where for the last inequality we have used that $8L^2\exp(-c\la^2/L^2R^2)\leq \frac{1}{2}$ is equivalent to 
$\la^2 \gtrsim R^2 L^2 \log(4L)$.
\end{proof}

\begin{theorem}[{\cite[Theorem 2.10]{dirksen_robust_2018}}]
\label{subgaussian_tail}
Let $\a_1, \ldots, \a_m$ denote independent, isotropic L-subgaussian random vectors and let $\S \subseteq \R^n$ . If $1\leq k \leq m$ and $u \geq 1$ then with probability at least $1 - 2 exp(-c_1 u^2 k \log(em/k))$, 
\begin{equation}
 \sup_{\x \in \S}  \max_{|I| \leq k} \Big( \sum_{i \in I} \inner{\a_i}{\x}^2 \Big)^{\frac{1}{2}}
 \leq c_2 \Big(\E \sup_{\x \in \S} |\inner{\g}{\x}| + u d_S \sqrt{k \log(em/k)} \Big)
\end{equation}
where $\g \sim \N(0,\text{id})$, $c_1$ and $c_2$ depend only on $L$ and $d_S = \sup_{\x\in \S} \norm{\x}{2}$.
\end{theorem}


\section{Alternative Proof of ...}

\begin{lemma}
Let $\ep, \rho>0$. Then with probability at least 
$1-\exp(-c\ep^2 m/\rho^2)$,
\begin{displaymath}
 \sup_{\z\in (\T-\T)\cap \ep B^n_2}|\{i\in [m]\; : \; |\inner{\a_i}{\z}|>\rho\}|\lesssim
 m \cdot  \Big(\frac{L w((\T-\T)\cap \ep B^n_2)}{\rho\sqrt{m}} + \frac{\ep}{\rho}\Big).
\end{displaymath}

\end{lemma}
\begin{proof} 
Using symmetrization and contraction, we obtain
 \begin{align*}
  \E\sup_{\z\in (\T-\T)\cap \ep B^n_2}|\{i\in [m]\; : \; |\inner{\a_i}{\z}|>\rho\}|
  &\leq \frac{1}{\rho} \E\sup_{\z\in (\T-\T)\cap \ep B^n_2}\sum_{i=1}^m |\inner{\a_i}{\z}|\\
  &\leq \frac{1}{\rho} \E\sup_{\z\in (\T-\T)\cap \ep B^n_2}\sum_{i=1}^m (|\inner{\a_i}{\z}|-\E|\inner{\a_i}{\z}|)\\
  &\quad + \frac{m\ep}{\rho}\\
  &\leq \frac{2}{\rho} \E\sup_{\z\in (\T-\T)\cap \ep B^n_2}\sum_{i=1}^m \ep_i |\inner{\a_i}{\z}|
   + \frac{m\ep}{\rho}\\
  &\leq \frac{2}{\rho} \E\sup_{\z\in (\T-\T)\cap \ep B^n_2}\sum_{i=1}^m \ep_i \inner{\a_i}{\z}
   + \frac{m\ep}{\rho},
 \end{align*}
 where $\ep_1, \ldots, \ep_m\in \{-1,1\}$ are independent Rademacher random variables.
 By Talagrand's majorizing measures theorem we know that 
 \begin{displaymath}
  \E\sup_{\z\in (\T-\T)\cap \ep B^n_2}\sum_{i=1}^m \ep_i \inner{\a_i}{\z}\lesssim L \cdot \sqrt{m} \cdot w((\T-\T)\cap \ep B^n_2).
 \end{displaymath}
In total,
\begin{displaymath}
 \E\sup_{\z\in (\T-\T)\cap \ep B^n_2}|\{i\in [m]\; : \; |\inner{\a_i}{\z}|>\rho\}|\lesssim 
 \frac{L\sqrt{m} w((\T-\T)\cap \ep B^n_2) + m \ep}{\rho}.
\end{displaymath}
The bounded difference inequality implies that for every $t>0$ with probability at least $1-\exp(-ct^2 m)$,
\begin{align*}
 \sup_{\z\in (\T-\T)\cap \ep B^n_2}|\{i\in [m]\; : \; |\inner{\a_i}{\z}|>\rho\}|
 &\leq \E\sup_{\z\in (\T-\T)\cap \ep B^n_2}|\{i\in [m]\; : \; |\inner{\a_i}{\z}|>\rho\}|\\
 &\quad + tm.
\end{align*}
Hence, for the choice $t=\frac{\ep}{\rho}$ we obtain that with probability at least 
$1-\exp(-c\ep^2 m/\rho^2)$,
\begin{displaymath}
 \sup_{\z\in (\T-\T)\cap \ep B^n_2}|\{i\in [m]\; : \; |\inner{\a_i}{\z}|>\rho\}|\lesssim
  \frac{L\sqrt{m} w((\T-\T)\cap \ep B^n_2)}{\rho} + \frac{m\ep}{\rho}.
\end{displaymath}
\end{proof}

\section{Old stuff \& to be deleted}
\begin{corollary} \label{lemma/positivity}
Let $\z \in RB_2^n$ and $\lambda \gg R$. Assume that $\rho/\lambda \leq 1$, $\T\subset R B^n_2$,
\begin{equation}
    \log|\N(\T,\norm{\cdot}{2},\ep)| \lesssim \frac{\rho}{\lambda}m, \quad\text{with} \quad
     \quad \ep \lesssim \frac{\rho}{\log(\lambda/\rho)} \; ,
\end{equation}
and
\begin{equation}
    m \gg \lambda \rho^{-3} w_*((\T-\T)\cap \ep B^n_2)^2 \; .
\end{equation}
Then, with probability exceeding 
\begin{displaymath}
 1- 2\exp\Big(-
 c m\frac{\rho}{\lambda}\Big) \; ,
\end{displaymath}
\begin{equation}
    \forall \x \in \T \setminus (\rho B_2^n + \z) \; :\;   
    \L_{q(\x)}(\z) \gg \frac{\norm{\x-\z}{2}^2}{\lambda} \; .
\end{equation}
\end{corollary}
This lemma implies the following result for a net in $\T$.
\begin{lemma}\label{lem:bound_on_net}
Let $\lambda \gg R$. Assume that $\rho/\lambda \leq 1$, $\T\subset R B^n_2$, and let $\N_\ep$ denote a $\ep$-net in $\T$ in the Euclidean metric. Suppose
\begin{equation}
    \log|\N_\ep| \lesssim \frac{\rho}{\lambda}m, \quad\text{with} \quad
     \quad \ep \lesssim \frac{\rho}{\log(\lambda/\rho)} \; ,
\end{equation}
and
\begin{equation}
    m \gg \lambda \rho^{-3} w_*((\T-\T)\cap \ep B^n_2)^2 \; .
\end{equation}
Then, with probability exceeding 
\begin{displaymath}
 1- 2\exp\Big(-
 c m\frac{\rho}{\lambda}\Big) \; ,
\end{displaymath}
\begin{equation}
    \forall \z' \in \N_\ep,\, \x\in \T \setminus (\rho B_2^n + \z') \; :\;   \L_{q(\x)}(\z') \gg \frac{\norm{\x-\z'}{2}^2}{\lambda}. \;
\end{equation}
\end{lemma}
\begin{proof}
Corollary \ref{lemma/positivity} shows that for each $\z'\in \N_\ep$ it holds
\begin{equation}
    \Pb\Big(\forall \x \in \T \setminus (\rho B_2^n + \z') \; :\;  
    \L_{q(\x)}(\z') \gg \frac{\norm{\x-\z'}{2}^2}{\lambda} \Big)\geq 1- 2\exp\Big(-
 c m\frac{\rho}{\lambda}\Big)\; .
\end{equation}
Since $\log |\N_\ep| \lesssim \frac{\rho}{\lambda} m$, it follows by a union bound that 
\begin{align*}
    \Pb \Big( \exists \z' \in \N_\ep\colon  \exists\x\in \T \setminus (\rho B_2^n + \z') &:
    \L_{q(\x)}(\z') \lesssim \frac{\norm{\x-\z}{2}^2}{ \lambda}  \Big) \\
    &\leq 2|\N_\ep| \exp(-m \rho/\lambda) \\
    &\lesssim \exp(-m \rho/\lambda) \; .
\end{align*}
This shows the assertion.
\end{proof}

\proof[of Theorem \ref{thm/positivity}] 
Let $\rho,\ep>0$ with $4\ep\leq \rho$, and let $\N_\ep$ be a $\ep$-cover of $\T$ with $\log |\N_\ep| \lesssim \frac{\rho}{\lambda} m$. Let $\x,\z\in \T$ with $\norm{\x-\z}{2} \geq 2\rho$. There exist $\z' \in \N_\ep$ such that $\norm{\z-\z'}{2} \leq \ep$. By the triangle inquality it follows $\|\x-\z'\|_2\geq \norm{\x-\z}{2}-\ep\geq  2\rho- \ep\geq \rho$.
In this situation we study the following decomposition of $\L_{q(\x)}(\z)$:
\begin{align*}
    \L_{q(\x)}(\z) 
&=\L_{q(\x)}(\z) - \L_{q(\x)}(\z') + \L_{q(\x)}(\z') \\
    &=\frac{1}{m} \sum_{i=1}^m \Big(\relu{- 
    \sign(\inner{\a_i}{\x} + \tau_i) (\inner{\a_i}{\z} + \tau_i)} \\
    &\qquad\qquad-\relu{-\sign(\inner{\a_i}{\x} + \tau_i) (\inner{\a_i}{\z'} + \tau_i)}\Big)\\
    &\quad +\L_{q(\x)}(\z')\\
    &\geq -\frac{1}{m} \sum_{i=1}^m \relu{- 
    \sign(\inner{\a_i}{\x} + \tau_i) (\inner{\a_i}{\z'-\z})}\\
    &\quad +\L_{q(\x)}(\z'),\\
\end{align*}
where we have used that for all $a,b\in \R$,
\begin{displaymath}
 \relu{a}-\relu{b}\geq - \relu{b-a}.
\end{displaymath}
Lemma \ref{lem:bound_on_net} implies for $\ep=c\frac{\rho^2}{\la}$ that with probability exceeding 
\begin{displaymath}
 1- 2\exp\Big(-
 c m\frac{\rho}{\lambda}\Big) \; ,
\end{displaymath}
\begin{equation}
    \forall \z' \in \N_\ep,\, \x\in \T \setminus (\rho B_2^n + \z') \; :\;   \L_{q(\x)}(\z') \gg \frac{\norm{\x-\z'}{2}^2}{\lambda}. \;
\end{equation}
Therefore, if we show that with high probability,  
\begin{equation}
\label{small_euclidean_distance}
\sup_{\x\in \T} \sup_{\z' \in \N_\ep, \z\in \T:\|\z-\z'\|_2\leq \ep}\frac{1}{m} \sum_{i=1}^m \relu{- 
    \sign(\inner{\a_i}{\x} + \tau_i) (\inner{\a_i}{\z'-\z})} \lesssim \ep,
\end{equation}
then the result follows.
We estimate using Cauchy-Schwarz: 
\begin{equation*}
\frac{1}{m} \sum_{i=1}^m \relu{- 
    \sign(\inner{\a_i}{\x} + \tau_i) (\inner{\a_i}{\z'-\z})}
    \leq \frac{1}{m} \sum_{i=1}^m |\inner{\a_i}{\z'-\z}| \leq \frac{1}{\sqrt{m}} \|\A(\z'-\z)\|_2.
\end{equation*}    
Hence, in order to control \eqref{small_euclidean_distance}, it suffices to bound
\begin{displaymath}
 \sup_{\z\in (\T-\T)\cap \ep B^n_2}\frac{1}{\sqrt{m}} \|\A\z\|_2.
\end{displaymath}
From \red{\cite[Exercise 9.1.8]{vershynin_hdp_2018}} it follows that for any $u>0$ with probability at least $1-2\exp(-u^2)$,
\begin{displaymath}
 \sup_{\z\in (\T-\T)\cap \ep B^n_2}\big|\frac{1}{\sqrt{m}} \|\A\z\|_2 -\|\z\|_2\big|\lesssim L^2 \cdot \frac{w((\T-\T)\cap \ep B^n_2) +u\ep}{\sqrt{m}}.
\end{displaymath}
Hence, for the choice $u=c \sqrt{m}/L^2$, we obtain that with probability at least $1-2\exp(-cm/L^4)$,
\begin{displaymath}
\sup_{\z\in (\T-\T)\cap \ep B^n_2}\big|\frac{1}{\sqrt{m}} \|\A\z\|_2 -\|\z\|_2\big|\lesssim \frac{ L^2 \cdot w((\T-\T)\cap \ep B^n_2) }{\sqrt{m}}+ \ep.
\end{displaymath}
Hence, if $m\gtrsim L^4 \cdot \ep^{-2}\cdot w((\T-\T)\cap \ep B^n_2)^2$, then with
probability at least $1-2\exp(-cm/L^4)$,
\begin{displaymath}
 \sup_{\z\in (\T-\T)\cap \ep B^n_2}\frac{1}{\sqrt{m}} \|\A\z\|_2\lesssim \ep.
\end{displaymath}
